# Supplementary material for: MeshVPR: Citywide Visual Place Recognition Using 3D Meshes
Source: arXiv:2406.02776 source file (2024-07-24)
Supplement: Supplementary file 1 [file X_suppl.tex]

\section{Training details}

\myparagraph{Pipeline's resources and time.}
\rzt{
Our training protocol employs San Francisco eXtra Large (SF-XL) \cite{Berton_2022_cosPlace} datasets and the San Francisco HQ mesh, accounting for 91GB of total storage, which required us $\approx 3h$ to download. The generation of synthetic samples corresponding to views of the real dataset takes $\approx 4h$ on a consumer PC, while the feature alignment step itself requires only $\approx 2h$ for a ResNet50-based model on an Nvidia GeForce RTX 4090.
Similarly, downloading the 3D mesh and generating the synthetic database took $\approx 9h$ for our Berlin dataset, which is the biggest one in this study. Details of required time for each step is depicted in \cref{fig:pipeline}.
}
\rz{Question for GB: inference time is different for MeshVPR and base method? I think we can simplify here, and say that from here on the cost is the same of the standard VPR. In both cases, at inference it should not be necessary to extract the database's features (can be done in advance).}
\gb{Yes the inference is the same. Might be worth mentioning though that it's fast (<0.01s per query)}

\subsection{Experimental Setting}
\myparagraph{Features Alignment.}
Our feature alignment is performed 
by pairing two copies of the same VPR model (\eg NetVLAD, CosPlace, MixVPR), both initialized with open-source pretrained weights.
One of the two models, which we refer to as $f_{\theta_{real}}$, has frozen weights $\theta_{real}$, while the weights $\theta_{synt}$ of $f_{\theta_{synt}}$ are fine-tuned for 50k iterations with a batch size of 32 and the Adam \cite{Kingma_2014_adam} optimizer with learning rate $1e-5$.
As per the training set, we use the largest publicly available VPR dataset, namely San Francisco eXtra Large (SF-XL) \cite{Berton_2022_cosPlace} and its 3D mesh counterpart, with synthetic views extracted from the San Francisco HQ mesh (see \cref{tab:3d_models}).

\myparagraph{Inference.}
At inference time, $f_{\theta_{synt}}$ is used to extract features from synthetic database, while the queries are processed through $f_{\theta_{real}}$. As in standard VPR \cite{Arandjelovic_2018_netvlad, Ge_2020_sfrs, Alibey_2022_gsvcities, Berton_2022_cosPlace, Alibey_2023_mixvpr, Berton_2023_EigenPlaces}, queries' features are matched against database ones by kNN algorithm (see \cref{fig:architecture}, right).

\subsection{Exploration of metric learning strategies.}
In this section we question the need for the two-models approach of MeshVPR, by understanding if a simpler pre-existing single-model technique could achieve competitive performances.
We investigate this by incorporating existing metric learning strategies, and training on a combination of real and synthetic data: one such example is the method employed in \cite{vallone2022danish}, where a Triplet loss takes triplets made of synthetic and real images.
To provide an exhaustive set of experiments, we show not only results with the methodology presented in \cite{vallone2022danish}, but with a large number of metric learning losses \cite{Song_2016_liftedLoss, vandenOord_2018_NTXentLoss_InfoNce, Cakir_2019_fastAP, Sun_2020_CircleLoss, Khosla_2020_SupCon}
conveniently implemented in the PyTorch Metric Learning library \cite{Musgrave_2020_PyTorchML}.
For each loss, we performed hyperparameters tuning to find the best values.
As training set, we use the overlapping datasets of San Francisco HQ (for synthetic) and SF-XL (for real images), which is the same training set used for MeshVPR.

%%%%%%%%%%%%%%%%%%%%%%%%%%%%%%%%%%%%%%%%%%%%%%%%%%%%%%%%%%%%%%%%

\input{tables/other_baselines}

\rzt{Results from \cref{tab:other_baselines} demonstrate that existing solutions do not provide an effective improvement over the base EigenPlaces method, which is the current best performing algorithm in standard VPR. Conversely, integrating it with MeshVPR pipeline outperforms other solutions by a large margin, thus demonstrating the benefit of MeshVPR's  two-models strategy, with one model extracting features from real images and the other extracting aligned features from synthetic images.  }

\subsection{Comparing MeshVPR with other strategies}
Results from \cref{tab:other_baselines} demonstrate the benefit of MeshVPR's  two-models strategy, with one model extracting features from real images and the other extracting aligned features from synthetic images.
On the other hand, other solutions only alleviate the problem and do not achieve competitive results with MeshVPR.
We note that this is partially in contrast with the findings of \cite{vallone2022danish},
which reports that \textit{the appearance differences between real and rendered images are not an issue when matching deep features}.
We believe this divergence in findings to be related to the size of the database: \cite{vallone2022danish} used a much smaller database of only 44k images, reducing the complexity of the task,
whereas we focus on challenging large-scale citywide databases with up to 30 times the number of images.

\section{Examples of Queries}
\label{sec:supp_queries}
Figures \ref{fig:q_sf}, \ref{fig:q_berlin}, \ref{fig:q_mel}, \ref{fig:q_paris} show examples of queries from San Francisco, Berlin, Melbourne and Paris.
\input{figures/q_sf}
\input{figures/q_berlin}
\input{figures/q_mel}
\input{figures/q_paris}

\section{Examples of Database Images}
\label{sec:supp_database}
Figures \ref{fig:db_sf}, \ref{fig:db_berlin}, \ref{fig:db_mel}, \ref{fig:db_paris} show examples of database synthetic images respectively from San Francisco, Berlin, Melbourne and Paris.
\input{figures/db_sf}
\input{figures/db_berlin}
\input{figures/db_mel}
\input{figures/db_paris}

\section{More Qualitative Results and Failure Cases}
\label{sec:supp_qualitative}
Figures \ref{fig:preds_sf}, \ref{fig:preds_berlin}, \ref{fig:preds_mel}, \ref{fig:preds_paris} show examples of prediction on synthetic dataset for a given query respectively from San Francisco, Berlin, Melbourne and Paris. Most of the times, predictions are qualitatively good and even in some failures the image retrieved are very similar to the query. Some failures can also be attributed to the low quality of the meshes or occlusions in the 3D scene, which means that as higher quality meshes become available the methods using MeshVPR will also improve. 
% However, synthetic images quality is an important factor, and occlusions hinder performances.
\input{figures/preds_supp_sf}
\input{figures/preds_supp_berlin}
\input{figures/preds_supp_mel}
\input{figures/preds_supp_paris}
